# Supplementary material for: SignSplat: Rendering Sign Language via Gaussian Splatting
Source: arXiv:2505.02108 source file (2025-05-04)
Supplement: Supplementary file 1 [file X_suppl.tex]

\section{Demos}
% We include two demo videos highlighting our approach.
% The first video ``sign\_stitching\_comparison.mp4'' (see Fig.~\ref{fig:gan_comparison}) shows comparison of our gloss stitching method and rendering with GAN approach by Saunders~{\etal}. In bottom of the image red colors label the method name, and in blue is the gloss name or transition.
% The second video ``novel\_views.mp4'' (see Fig.~\ref{fig:novel_view}) demonstrates skeleton, point cloud, Gaussian splatting rendering, and CNN improvement across novel views.

We include a demo video (``sign\_stitching\_comparison.mp4'') to showcase our approach for gloss stitching. Fig.~\ref{fig:gan_comparison} compares our gloss stitching method with the GAN-based rendering approach by Saunders~{\etal}~\cite{SaundersBen2020ESNT} The bottom of the image highlights the method name in red and the gloss name or transition in blue.

% \begin{enumerate}
%     \item ``novel\_views.mp4'' -- shows renderings of circular motion around 3D Gaussian splats.
%     \item ``sign\_stitching\_comprison.mp4'' -- shows a comparison of our renderings against the GAN output. The red subtitles on the top-right part of the video provide the name of the gloss and the transition between the two glosses. 
% \end{enumerate}  

% \vspace{-1cm}
\begin{figure}[!htbp]
    \centering
    \includegraphics[width=0.99\linewidth]{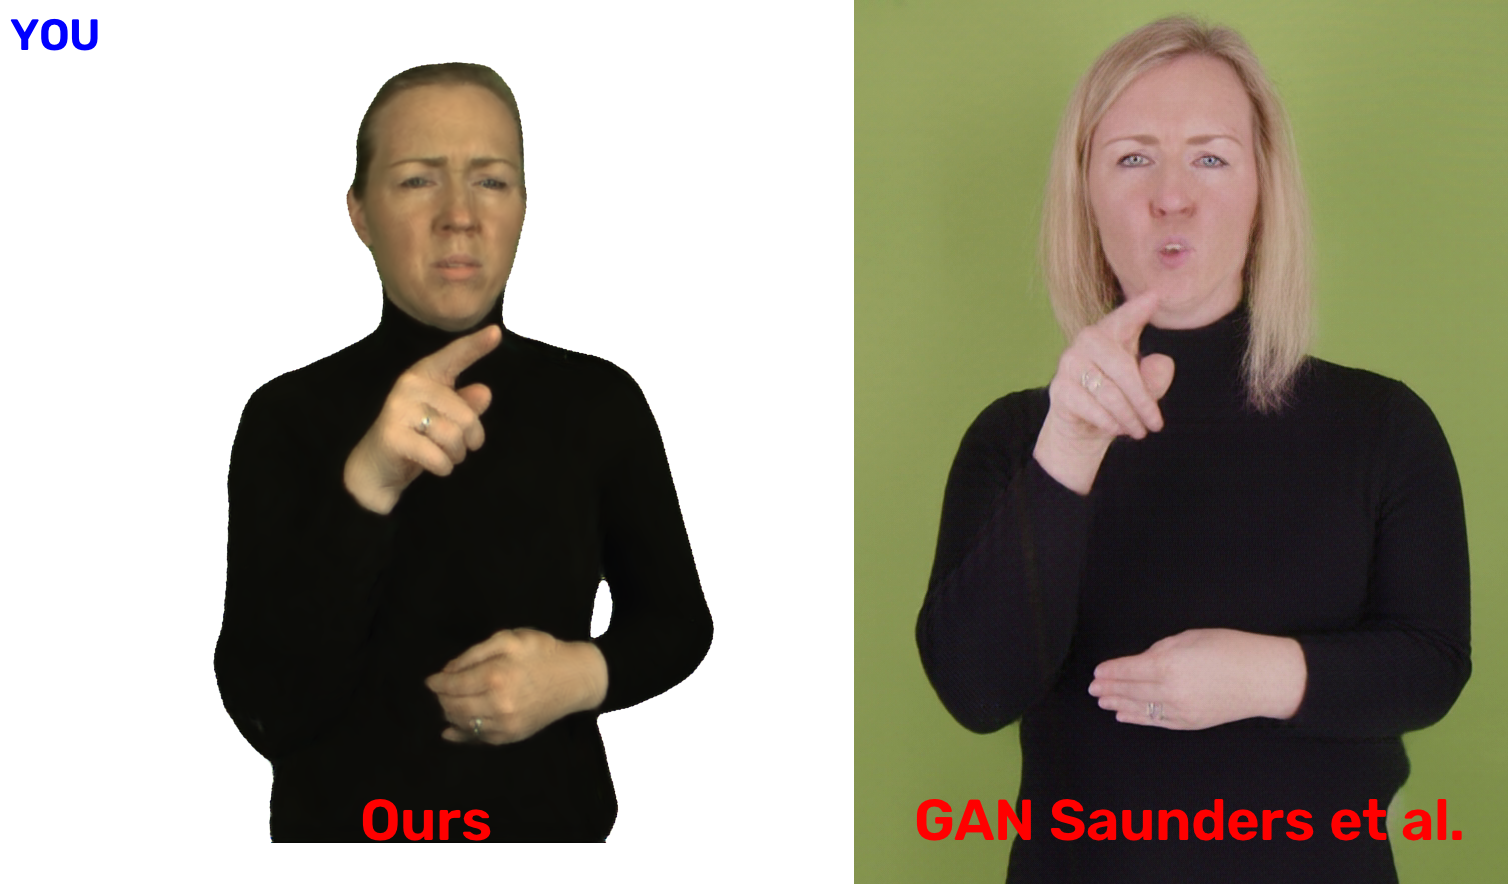}
    \caption{Comparison of our rendering versus GAN of Saunders~{\etal}}
    \label{fig:gan_comparison}
\end{figure}
